# Supplementary material for: Leveraging secondary-structure information for accurate nucleic acid structure prediction with OFoldNA
Source: arXiv:2609.37414 source file (2026-10-08)
Supplement: Supplementary file 1 [file 00_preface.tex]

[Appendix preface or supplementary-material note.]
