# Supplementary material for: Leveraging secondary-structure information for accurate nucleic acid structure prediction with OFoldNA
Source: arXiv:2609.37414 source file (2026-10-08)
Supplement: Supplementary file 2 [file 02_appendix.tex]

\section{[Appendix section title]}

[Appendix content.]
